# Supplementary material for: Secure and Robust MIMO Transceiver for Multicast Mission Critical Communications
Source: arXiv:2012.05829 source file (2020-12-10)
Supplement: Supplementary file 1 [file appendix_norm_bounded.tex]

Problem B: Computation of worst case channels, i.e., Computation of worst case channels/ channel vectors that belong to the uncertainty region and minimize total legitimate users mean square error.

\begin{eqnarray}
&&\min_{{\bf \Delta}_{ie} \forall 1 \leq i \leq K1} \epsilon_{e} \\
&&\text{s.t.} \nonumber \\
&& ||{\bf \Delta}_{ie}||^{2} \leq \sigma_{ie} \quad \forall 1 \leq i \leq K1 \nonumber
\end{eqnarray}
Where MSE at eve-dropper with channel errors can be written as:
\begin{eqnarray}
&&\epsilon_{e} = tr\bigg(I-\sum_{i=1}^{K_1}{\bf V}_{i}^{H}{\bf G}_{ie}^{H}{\bf E}_{e}^{H} - \sum_{i=1}^{K_1}{\bf E}_{e}{\bf G}_{ie}{\bf V}_{i}  + \sum_{i=1}^{K_1}{\bf E}_{e}{\bf G}_{ie}{\bf V}_{i}{\bf V}_{i}^{H}{\bf G}_{ie}^{H}{\bf E}_{e}^{H} \nonumber \\
&& + \sum_{i=1}^{K_1}{\bf E}_{e}{\bf G}_{ie}{\bf W}_{i}{\bf G}_{ie}^{H}{\bf E}_{e}^{H} + \sigma_{ne}^{2}{\bf E}_{e}{\bf E}_{e}^{H}\bigg) \nonumber \\
&&= tr\bigg(I-\sum_{i=1}^{K_1}{\bf V}_{i}^{H}(\widehat{{\bf G}}_{ie}+{\bf \Delta}_{ie})^{H}{\bf E}_{e}^{H} - \sum_{i=1}^{K_1}{\bf E}_{e}(\widehat{{\bf G}}_{ie}+{\bf \Delta}_{ie}){\bf V}_{i} \nonumber \\
&& + \sum_{i=1}^{K_1}{\bf E}_{e}(\widehat{{\bf G}}_{ie}+{\bf \Delta}_{ie}){\bf V}_{i}{\bf V}_{i}^{H}(\widehat{{\bf G}}_{ie}+{\bf \Delta}_{ie})^{H}{\bf E}_{e}^{H} + \sum_{i=1}^{K_1}{\bf E}_{e}(\widehat{{\bf G}}_{ie}+{\bf \Delta}_{ie}){\bf W}_{i}(\widehat{{\bf G}}_{ie}+{\bf \Delta}_{ie})^{H}{\bf E}_{e}^{H} + \sigma_{ne}^{2}{\bf E}_{e}{\bf E}_{e}^{H}\bigg) \nonumber \\
&&= tr\bigg(I-\sum_{i=1}^{K_1}{\bf V}_{i}^{H}\widehat{{\bf G}}_{ie}^{H}{\bf E}_{e}^{H} - \sum_{i=1}^{K_1}{\bf E}_{e}\widehat{{\bf G}}_{ie}{\bf V}_{i} -\sum_{i=1}^{K_1}{\bf V}_{i}^{H}{\bf \Delta}_{ie}^{H}{\bf E}_{e}^{H} - \sum_{i=1}^{K_1}{\bf E}_{e}{\bf \Delta}_{ie}{\bf V}_{i} + \sum_{i=1}^{K_1}{\bf E}_{e}\widehat{{\bf G}}_{ie}{\bf V}_{i}{\bf V}_{i}^{H}\widehat{{\bf G}}_{ie}^{H}{\bf E}_{e}^{H} \nonumber \\
&&  + \sum_{i=1}^{K_1}{\bf E}_{e}\widehat{{\bf G}}_{ie}{\bf V}_{i}{\bf V}_{i}^{H}{\bf \Delta}_{ie}^{H}{\bf E}_{e}^{H} + \sum_{i=1}^{K_1}{\bf E}_{e}{\bf \Delta}_{ie}{\bf V}_{i}{\bf V}_{i}^{H}\widehat{{\bf G}}_{ie}^{H}{\bf E}_{e}^{H} + \sum_{i=1}^{K_1}{\bf E}_{e}{\bf \Delta}_{ie}{\bf V}_{i}{\bf V}_{i}^{H}{\bf \Delta}_{ie}^{H}{\bf E}_{e}^{H} + \sum_{i=1}^{K_1}{\bf E}_{e}\widehat{{\bf G}}_{ie}{\bf W}_{i}\widehat{{\bf G}}_{ie}^{H}{\bf E}_{e}^{H}   \nonumber \\
&&  + \sum_{i=1}^{K_1}{\bf E}_{e}\widehat{{\bf G}}_{ie}{\bf W}_{i}{\bf \Delta}_{ie}^{H}{\bf E}_{e}^{H} + \sum_{i=1}^{K_1}{\bf E}_{e}{\bf \Delta}_{ie}{\bf W}_{i}\widehat{{\bf G}}_{ie}^{H}{\bf E}_{e}^{H} + \sum_{i=1}^{K_1}{\bf E}_{e}{\bf \Delta}_{ie}{\bf W}_{i}{\bf \Delta}_{ie}^{H}{\bf E}_{e}^{H} + \sigma_{ne}^{2}{\bf E}_{e}{\bf E}_{e}^{H}\bigg)
\end{eqnarray}

For simplicity, we discard the second and higher order terms of ${\bf \Delta}_{ie}$. Also, let $\overline{\epsilon}_{e}$ represents the MSE at eves-dropper considering ${\bf \Delta}_{ie}$ to be zero. Hence, estimation of MSE caused by a specific BS can be written as:

\begin{eqnarray}
\epsilon_{ie} &\approx& \overline{\epsilon}_{ie} - tr({\bf V}_{i}^{H}{\bf \Delta}_{ie}^{H}{\bf E}_{e}^{H}) - tr({\bf E}_{e}{\bf \Delta}_{ie}{\bf V}_{i}) + tr({\bf E}_{e}\widehat{{\bf G}}_{ie}{\bf V}_{i}{\bf V}_{i}^{H}{\bf \Delta}_{ie}^{H}{\bf E}_{e}^{H}) + tr({\bf E}_{e}{\bf \Delta}_{ie}{\bf V}_{i}{\bf V}_{i}^{H}\widehat{{\bf G}}_{ie}^{H}{\bf E}_{e}^{H}) \nonumber \\
&&+ tr({\bf E}_{e}\widehat{{\bf G}}_{ie}{\bf W}_{i}{\bf \Delta}_{ie}^{H}{\bf E}_{e}^{H}) + tr({\bf E}_{e}{\bf \Delta}_{ie}{\bf W}_{i}\widehat{{\bf G}}_{ie}^{H}{\bf E}_{e}^{H})
\end{eqnarray}
Reformulating only the part of MSE with ${\bf \Delta}_{ie}$.
\begin{eqnarray}
\label{eq:mse_eve_appx}
\epsilon_{ie} &\approx& \overline{\epsilon}_{ie} - tr(({\bf V}_{i}{\bf E}_{e}{\bf \Delta}_{ie}) + ({\bf V}_{i}{\bf E}_{e}{\bf \Delta}_{ie})^{H}) + tr({\bf E}_{e}\widehat{{\bf G}}_{ie}({\bf V}_{i}{\bf V}_{i}^{H} + {\bf W}_{i}){\bf \Delta}_{ie}^{H}{\bf E}_{e}^{H})  \nonumber \\
&&+ tr({\bf E}_{e}{\bf \Delta}_{ie}({\bf V}_{i}{\bf V}_{i}^{H} + {\bf W}_{i})\widehat{{\bf G}}_{ie}^{H}{\bf E}_{e}^{H}) \nonumber \\
&\approx& \overline{\epsilon}_{ie} - tr(({\bf V}_{i}{\bf E}_{e}{\bf \Delta}_{ie}) + ({\bf V}_{i}{\bf E}_{e}{\bf \Delta}_{ie})^{H}) + tr((\widehat{{\bf G}}_{ie}^{H}{\bf E}_{e}^{H}{\bf E}_{e}{\bf \Delta}_{ie})^{H}({\bf V}_{i}{\bf V}_{i}^{H} + {\bf W}_{i}))  \nonumber \\
&&+ tr((\widehat{{\bf G}}_{ie}^{H}{\bf E}_{e}^{H}{\bf E}_{e}{\bf \Delta}_{ie})({\bf V}_{i}{\bf V}_{i}^{H} + {\bf W}_{i})) \nonumber \\
&\approx& \overline{\epsilon}_{ie} - tr(({\bf V}_{i}{\bf E}_{e}{\bf \Delta}_{ie}) + ({\bf V}_{i}{\bf E}_{e}{\bf \Delta}_{ie})^{H}) + tr(((\widehat{{\bf G}}_{ie}^{H}{\bf E}_{e}^{H}{\bf E}_{e}{\bf \Delta}_{ie})^{H} + (\widehat{{\bf G}}_{ie}^{H}{\bf E}_{e}^{H}{\bf E}_{e}{\bf \Delta}_{ie}))({\bf V}_{i}{\bf V}_{i}^{H} + {\bf W}_{i}))  \nonumber \\
\end{eqnarray}
Using the inner product and Cauchy-inequality properties of trace
\begin{eqnarray}
[tr(((\widehat{{\bf G}}_{ie}^{H}{\bf E}_{e}^{H}{\bf E}_{e}{\bf \Delta}_{ie})^{H} &+& (\widehat{{\bf G}}_{ie}^{H}{\bf E}_{e}^{H}{\bf E}_{e}{\bf \Delta}_{ie}))({\bf V}_{i}{\bf V}_{i}^{H} + {\bf W}_{i}))]^{2} \leq \nonumber \\
&&[tr(((\widehat{{\bf G}}_{ie}^{H}{\bf E}_{e}^{H}{\bf E}_{e}{\bf \Delta}_{ie})^{H} + (\widehat{{\bf G}}_{ie}^{H}{\bf E}_{e}^{H}{\bf E}_{e}{\bf \Delta}_{ie})))]^{2} [tr({\bf V}_{i}{\bf V}_{i}^{H} + {\bf W}_{i})]^{2} \nonumber
\end{eqnarray}
taking square root on both the sides
\begin{eqnarray}
tr(((\widehat{{\bf G}}_{ie}^{H}{\bf E}_{e}^{H}{\bf E}_{e}{\bf \Delta}_{ie})^{H} &+& (\widehat{{\bf G}}_{ie}^{H}{\bf E}_{e}^{H}{\bf E}_{e}{\bf \Delta}_{ie}))({\bf V}_{i}{\bf V}_{i}^{H} + {\bf W}_{i})) \leq \nonumber \\
&&tr(((\widehat{{\bf G}}_{ie}^{H}{\bf E}_{e}^{H}{\bf E}_{e}{\bf \Delta}_{ie})^{H} + (\widehat{{\bf G}}_{ie}^{H}{\bf E}_{e}^{H}{\bf E}_{e}{\bf \Delta}_{ie}))) tr({\bf V}_{i}{\bf V}_{i}^{H} + {\bf W}_{i}) \nonumber
\end{eqnarray}
Considering the worst-case solution
\begin{eqnarray}
tr(((\widehat{{\bf G}}_{ie}^{H}{\bf E}_{e}^{H}{\bf E}_{e}{\bf \Delta}_{ie})^{H} &+& (\widehat{{\bf G}}_{ie}^{H}{\bf E}_{e}^{H}{\bf E}_{e}{\bf \Delta}_{ie}))({\bf V}_{i}{\bf V}_{i}^{H} + {\bf W}_{i})) = \nonumber \\
&&tr(((\widehat{{\bf G}}_{ie}^{H}{\bf E}_{e}^{H}{\bf E}_{e}{\bf \Delta}_{ie})^{H} + (\widehat{{\bf G}}_{ie}^{H}{\bf E}_{e}^{H}{\bf E}_{e}{\bf \Delta}_{ie}))) tr({\bf V}_{i}{\bf V}_{i}^{H} + {\bf W}_{i}) \nonumber
\end{eqnarray}
Hence replacing in eqn \ref{eq:mse_eve_appx}, we get
\begin{eqnarray}
&\approx& \overline{\epsilon}_{ie} - tr(({\bf V}_{i}{\bf E}_{e}{\bf \Delta}_{ie}) + ({\bf V}_{i}{\bf E}_{e}{\bf \Delta}_{ie})^{H}) + tr(((\widehat{{\bf G}}_{ie}^{H}{\bf E}_{e}^{H}{\bf E}_{e}{\bf \Delta}_{ie})^{H} + (\widehat{{\bf G}}_{ie}^{H}{\bf E}_{e}^{H}{\bf E}_{e}{\bf \Delta}_{ie}))) tr({\bf V}_{i}{\bf V}_{i}^{H} + {\bf W}_{i}) \nonumber
\end{eqnarray}
Considering only the Real value from the equation, we can say that
\begin{eqnarray}
\mathbb{R}({\bf A})^{H} &=& \mathbb{R}({\bf A})^{T} \nonumber \\
\mathbb{R}tr({\bf A}) &=& \mathbb{R}tr({\bf A}^{T}) = \mathbb{R}tr({\bf A}^{H}) \nonumber
\end{eqnarray}
Hence, the MSE estimate can be written as:
\begin{eqnarray}
&\approx& \overline{\epsilon}_{ie} - 2\mathbb{R}tr({\bf V}_{i}{\bf E}_{e}{\bf \Delta}_{ie}) + 2\mathbb{R}tr(\widehat{{\bf G}}_{ie}^{H}{\bf E}_{e}^{H}{\bf E}_{e}{\bf \Delta}_{ie})tr({\bf V}_{i}{\bf V}_{i}^{H} + {\bf W}_{i}) \nonumber \\
&\approx& \overline{\epsilon}_{ie} + 2\mathbb{R}tr((B\widehat{{\bf G}}_{ie}^{H}{\bf E}_{e}^{H} - {\bf V}_{i}){\bf E}_{e}{\bf \Delta}_{ie})
\end{eqnarray}
where $B = tr({\bf V}_{i}{\bf V}_{i}^{H} + {\bf W}_{i})$, Using Cauchy-inequalities and solving it for worst case scenario
\begin{eqnarray}
{\bf \Delta}_{ie} = \frac{\sigma_{ie}}{||{\bf E}_{e}^{H}(B{\bf E}_{e}\widehat{{\bf G}}_{ie} -  {\bf V}_{i}^{H})||} (B{\bf E}_{e}\widehat{{\bf G}}_{ie} -  {\bf V}_{i}^{H})
\end{eqnarray}
