# Supplementary material for: Secure and Robust MIMO Transceiver for Multicast Mission Critical Communications
Source: arXiv:2012.05829 source file (2020-12-10)
Supplement: Supplementary file 2 [file appendix_convergence_proof.tex]

Proof for convergence of iterative algorithm.
