# Supplementary material for: Secure and Robust MIMO Transceiver for Multicast Mission Critical Communications
Source: arXiv:2012.05829 source file (2020-12-10)
Supplement: Supplementary file 3 [file appendix_mse.tex]

In this section, we formulate the MSE for both legitimate users and eavesdroppers. We formulate both the MSE while considering imperfections in the CSI at the BSs. Later, a generic equation for MSE is provided by incorporating two binary flags ${\chi}_{l}$ and ${\chi}_{e}$ into it. By changing the values of these flags, effective MSE for different scenarios can be formed.

\subsection{MSE at legitimate users}
The MSE at the legitimate users is computed as:
\begin{IEEEeqnarray}{lll}
\label{eq:mse_leg_complete}
{\epsilon}_{l} &=& \mathbb{E}\bigg[||\bf{d}-\widehat{\bf{d}}_{l}||^{2}\bigg] \nonumber
\\
&=& \mathbb {E}\bigg[||{\bf d}-(%
\sum_{t=1}^{K_T}{\bf R}_{l}(\widehat{\bf C}_{tl} + \boldsymbol{\Delta}_{tl}){\bf V}_{t}{\bf d} +%
\sum_{t=1}^{K_T}{\bf R}_{l}(\widehat{\bf C}_{tl} + \boldsymbol{\Delta}_{tl}){\bf w}_{t} +%
{\bf R}_{l}{\bf n}_{l}%
)||^{2}\bigg]\nonumber \\
&=& \mathbb {E}\bigg[{\rm tr}\Big(({\bf d}-(%
\sum_{t=1}^{K_T}{\bf R}_{l}(\widehat{\bf C}_{tl} + \boldsymbol{\Delta}_{tl}){\bf V}_{t}{\bf d} +%
\sum_{t=1}^{K_T}{\bf R}_{l}(\widehat{\bf C}_{tl} + \boldsymbol{\Delta}_{tl}){\bf w}_{t} +%
{\bf R}_{l}{\bf n}_{l}%
)) \nonumber \\
&& \qquad ({\bf d}-(%
\sum_{t=1}^{K_T}{\bf R}_{l}(\widehat{\bf C}_{tl} + \boldsymbol{\Delta}_{tl}){\bf V}_{t}{\bf d} +%
\sum_{t=1}^{K_T}{\bf R}_{l}(\widehat{\bf C}_{tl} + \boldsymbol{\Delta}_{tl}){\bf w}_{t} +%
{\bf R}_{l}{\bf n}_{l}%
))^{H}\Big)\bigg]\nonumber \\
&=& \mathbb{E}\bigg[{\rm tr}\Big(%
{\bf d}{\bf d}^{H}-%
\sum_{t=1}^{K_T}{\bf R}_{l}(\widehat{\bf C}_{tl} + \boldsymbol{\Delta}_{tl}){\bf V}_{t}{\bf d}{\bf d}^{H} -%
\sum_{t=1}^{K_T}{\bf R}_{l}(\widehat{\bf C}_{tl} + \boldsymbol{\Delta}_{tl}){\bf w}_{t}{\bf d}^{H} -%
{\bf R}_{l}{\bf n}_{l}{\bf d}^{H} - \nonumber \\%
&&\quad \sum_{t=1}^{K_T}{\bf d}{\bf d}^{H}{\bf V}_{t}^{H}(\widehat{\bf C}_{tl} + \boldsymbol{\Delta}_{tl})^{H}{\bf R}_{l}^{H} +%
\sum_{t=1}^{K_T}{\bf R}_{l}(\widehat{\bf C}_{tl} + \boldsymbol{\Delta}_{tl}){\bf V}_{t}{\bf d}{\bf d}^{H}{\bf V}_{t}^{H}(\widehat{\bf C}_{tl} + \boldsymbol{\Delta}_{tl})^{H}{\bf R}_{l}^{H} \nonumber \\%
&&+ \sum_{t=1}^{K_T}{\bf R}_{l}(\widehat{\bf C}_{tl} + \boldsymbol{\Delta}_{tl}){\bf w}_{t}{\bf d}^{H}{\bf V}_{t}^{H}(\widehat{\bf C}_{tl} + \boldsymbol{\Delta}_{tl})^{H}{\bf R}_{l}^{H} +%
\sum_{t=1}^{K_T}{\bf R}_{l}{\bf n}_{l}{\bf d}^{H}{\bf V}_{t}^{H}(\widehat{\bf C}_{tl} + \boldsymbol{\Delta}_{tl})^{H}{\bf R}_{l}^{H} \nonumber \\%
&&- \sum_{t=1}^{K_T}{\bf d}{\bf w}_{t}^{H}(\widehat{\bf C}_{tl} + \boldsymbol{\Delta}_{tl})^{H}{\bf R}_{l}^{H} +%
\sum_{t=1}^{K_T}{\bf R}_{l}(\widehat{\bf C}_{tl} + \boldsymbol{\Delta}_{tl}){\bf V}_{t}{\bf d}{\bf w}_{t}^{H}(\widehat{\bf C}_{tl} + \boldsymbol{\Delta}_{tl})^{H}{\bf R}_{l}^{H} + \nonumber \\%
&&\quad \sum_{t=1}^{K_T}{\bf R}_{l}(\widehat{\bf C}_{tl} + \boldsymbol{\Delta}_{tl}){\bf w}_{t}{\bf w}_{t}^{H}(\widehat{\bf C}_{tl} + \boldsymbol{\Delta}_{tl})^{H}{\bf R}_{l}^{H} +%
\sum_{t=1}^{K_T}{\bf R}_{l}{\bf n}_{l}{\bf w}_{t}^{H}(\widehat{\bf C}_{tl} + \boldsymbol{\Delta}_{tl})^{H}{\bf R}_{l}^{H} - \nonumber \\
&&\quad {\bf d}{\bf n}_{l}^{H}{\bf R}_{l}^{H} +% \sum_{t=1}^{K_T}{\bf R}_{l}(\widehat{\bf C}_{tl} + \boldsymbol{\Delta}_{tl}){\bf V}_{t}{\bf d}{\bf n}_{l}^{H}{\bf R}_{l}^{H} +%
\sum_{t=1}^{K_T}{\bf R}_{l}(\widehat{\bf C}_{tl} + \boldsymbol{\Delta}_{tl}){\bf w}_{t}{\bf n}_{l}^{H}{\bf R}_{l}^{H} +%
{\bf R}_{l}{\bf n}_{l}{\bf n}_{l}^{H}{\bf R}_{l}^{H}%
\Big)\bigg]\nonumber \\
&=& \mathbb{E}\bigg[{\rm tr}\Big(%
{\bf d}{\bf d}^{H}-%
\sum_{t=1}^{K_T}{\bf R}_{l}\widehat{\bf C}_{tl}{\bf V}_{t}{\bf d}{\bf d}^{H} -%
\sum_{t=1}^{K_T}{\bf R}_{l}\boldsymbol{\Delta}_{tl}{\bf V}_{t}{\bf d}{\bf d}^{H} -%
\sum_{t=1}^{K_T}{\bf R}_{l}\widehat{\bf C}_{tl}{\bf w}_{t}{\bf d}^{H} - \nonumber \\%
&&\quad \sum_{t=1}^{K_T}{\bf R}_{l}\boldsymbol{\Delta}_{tl}{\bf w}_{t}{\bf d}^{H} -% 
{\bf R}_{l}{\bf n}_{l}{\bf d}^{H} -%
\sum_{t=1}^{K_T}{\bf d}{\bf d}^{H}{\bf V}_{t}^{H}\widehat{\bf C}_{tl}^{H}{\bf R}_{l}^{H} +%
\sum_{t=1}^{K_T}{\bf d}{\bf d}^{H}{\bf V}_{t}^{H}\boldsymbol{\Delta}_{tl}^{H}{\bf R}_{l}^{H} + \nonumber \\
&&\quad \sum_{t=1}^{K_T}{\bf R}_{l}\widehat{\bf C}_{tl}{\bf V}_{t}{\bf d}{\bf d}^{H}{\bf V}_{t}^{H}\widehat{\bf C}_{tl}^{H}{\bf R}_{l}^{H} +%
\sum_{t=1}^{K_T}{\bf R}_{l}\widehat{\bf C}_{tl}{\bf V}_{t}{\bf d}{\bf d}^{H}{\bf V}_{t}^{H}\boldsymbol{\Delta}_{tl}^{H}{\bf R}_{l}^{H} +\nonumber \\%
&&\quad \sum_{t=1}^{K_T}{\bf R}_{l}\boldsymbol{\Delta}_{tl}{\bf V}_{t}{\bf d}{\bf d}^{H}{\bf V}_{t}^{H}\widehat{\bf C}_{tl}^{H}{\bf R}_{l}^{H} +%
\sum_{t=1}^{K_T}{\bf R}_{l}\boldsymbol{\Delta}_{tl}{\bf V}_{t}{\bf d}{\bf d}^{H}{\bf V}_{t}^{H}\boldsymbol{\Delta}_{tl}^{H}{\bf R}_{l}^{H} + \nonumber \\%
&&\quad \sum_{t=1}^{K_T}{\bf R}_{l}\widehat{\bf C}_{tl}{\bf w}_{t}{\bf d}^{H}{\bf V}_{t}^{H}\widehat{\bf C}_{tl}^{H}{\bf R}_{l}^{H} +%
\sum_{t=1}^{K_T}{\bf R}_{l}\widehat{\bf C}_{tl}{\bf w}_{t}{\bf d}^{H}{\bf V}_{t}^{H}\boldsymbol{\Delta}_{tl}^{H}{\bf R}_{l}^{H} +\nonumber \\%
&&\quad \sum_{t=1}^{K_T}{\bf R}_{l}\boldsymbol{\Delta}_{tl}{\bf w}_{t}{\bf d}^{H}{\bf V}_{t}^{H}\widehat{\bf C}_{tl}^{H}{\bf R}_{l}^{H} +%
\sum_{t=1}^{K_T}{\bf R}_{l}\boldsymbol{\Delta}_{tl}{\bf w}_{t}{\bf d}^{H}{\bf V}_{t}^{H}\boldsymbol{\Delta}_{tl}^{H}{\bf R}_{l}^{H} +%
\sum_{t=1}^{K_T}{\bf R}_{l}{\bf n}_{l}{\bf d}^{H}{\bf V}_{t}^{H}\widehat{\bf C}_{tl}^{H}{\bf R}_{l}^{H} \nonumber \\
&&+ \sum_{t=1}^{K_T}{\bf R}_{l}{\bf n}_{l}{\bf d}^{H}{\bf V}_{t}^{H}\boldsymbol{\Delta}_{tl}^{H}{\bf R}_{l}^{H} -%
\sum_{t=1}^{K_T}{\bf d}{\bf w}_{t}^{H}\widehat{\bf C}_{tl}^{H}{\bf R}_{l}^{H} -%
\sum_{t=1}^{K_T}{\bf d}{\bf w}_{t}^{H}\boldsymbol{\Delta}_{tl}^{H}{\bf R}_{l}^{H} + \nonumber \\%
&&\quad \sum_{t=1}^{K_T}{\bf R}_{l}\widehat{\bf C}_{tl}{\bf V}_{t}{\bf d}{\bf w}_{t}^{H}\widehat{\bf C}_{tl}^{H}{\bf R}_{l}^{H} +%
\sum_{t=1}^{K_T}{\bf R}_{l}\widehat{\bf C}_{tl}{\bf V}_{t}{\bf d}{\bf w}_{t}^{H}\boldsymbol{\Delta}_{tl}^{H}{\bf R}_{l}^{H} +%
\sum_{t=1}^{K_T}{\bf R}_{l}\boldsymbol{\Delta}_{tl}{\bf V}_{t}{\bf d}{\bf w}_{t}^{H}\widehat{\bf C}_{tl}^{H}{\bf R}_{l}^{H} + \nonumber \\%
&&\quad \sum_{t=1}^{K_T}{\bf R}_{l}\boldsymbol{\Delta}_{tl}{\bf V}_{t}{\bf d}{\bf w}_{t}^{H}\boldsymbol{\Delta}_{tl}^{H}{\bf R}_{l}^{H} +%
\sum_{t=1}^{K_T}{\bf R}_{l}\widehat{\bf C}_{tl}{\bf w}_{t}{\bf w}_{t}^{H}\widehat{\bf C}_{tl}^{H}{\bf R}_{l}^{H} +%
\sum_{t=1}^{K_T}{\bf R}_{l}\widehat{\bf C}_{tl}{\bf w}_{t}{\bf w}_{t}^{H}\boldsymbol{\Delta}_{tl}^{H}{\bf R}_{l}^{H} + \nonumber \\%
&& \quad \sum_{t=1}^{K_T}{\bf R}_{l}\boldsymbol{\Delta}_{tl}{\bf w}_{t}{\bf w}_{t}^{H}\widehat{\bf C}_{tl}^{H}{\bf R}_{l}^{H} +%
\sum_{t=1}^{K_T}{\bf R}_{l}\boldsymbol{\Delta}_{tl}{\bf w}_{t}{\bf w}_{t}^{H}\boldsymbol{\Delta}_{tl}^{H}{\bf R}_{l}^{H} +%
\sum_{t=1}^{K_T}{\bf R}_{l}{\bf n}_{l}{\bf w}_{t}^{H}\widehat{\bf C}_{tl}^{H}{\bf R}_{l}^{H} + \nonumber \\%
&&\quad \sum_{t=1}^{K_T}{\bf R}_{l}{\bf n}_{l}{\bf w}_{t}^{H}\boldsymbol{\Delta}_{tl}^{H}{\bf R}_{l}^{H} -%
{\bf d}{\bf n}_{l}^{H}{\bf R}_{l}^{H} +%
\sum_{t=1}^{K_T}{\bf R}_{l}\widehat{\bf C}_{tl}{\bf V}_{t}{\bf d}{\bf n}_{l}^{H}{\bf R}_{l}^{H} +%
\sum_{t=1}^{K_T}{\bf R}_{l}\boldsymbol{\Delta}_{tl}{\bf V}_{t}{\bf d}{\bf n}_{l}^{H}{\bf R}_{l}^{H} + \nonumber \\%
&&\quad \sum_{t=1}^{K_T}{\bf R}_{l}\widehat{\bf C}_{tl}{\bf w}_{t}{\bf n}_{l}^{H}{\bf R}_{l}^{H} +%
\sum_{t=1}^{K_T}{\bf R}_{l}\boldsymbol{\Delta}_{tl}{\bf w}_{t}{\bf n}_{l}^{H}{\bf R}_{l}^{H} +%
{\bf R}_{l}{\bf n}_{l}{\bf n}_{l}^{H}{\bf R}_{l}^{H}%
\Big)\bigg]\nonumber
\end{IEEEeqnarray}
Now, we evaluate the expectation for all the terms using the properties of all variables as discussed in Sec.~\ref{sec:system_model}. Hence, the updated equation is formulated as:
\begin{IEEEeqnarray}{lll}
&=& {\rm tr}({\bf I}) -%
{\rm tr}(\sum_{t=1}^{K_T}{\bf R}_{l}\widehat{\bf C}_{tl}{\bf V}_{t}) -%
{\rm tr}(\sum_{t=1}^{K_T}{\bf V}_{t}^{H}\widehat{\bf C}_{tl}^{H}{\bf R}_{l}^{H}) +%
{\rm tr}(\sum_{t=1}^{K_T}{\bf R}_{l}\widehat{\bf C}_{tl}{\bf V}_{t}{\bf V}_{t}^{H}\widehat{\bf C}_{tl}^{H}{\bf R}_{l}^{H}) + \nonumber \\%
&&\quad {\rm tr}(\sum_{t=1}^{K_T}{\bf R}_{l}\widehat{\bf C}_{tl}{\bf W}_{t}\widehat{\bf C}_{tl}^{H}{\bf R}_{l}^{H}) +%
{\sigma}_{nl}^{2}{\rm tr}({\bf R}_{l}{\bf R}_{l}^{H}) +%
\mathbb{E}\big[{\rm tr}(\sum_{t=1}^{K_T}{\bf R}_{l}\boldsymbol{\Delta}_{tl}{\bf V}_{t}{\bf V}_{t}^{H}\boldsymbol{\Delta}_{tl}^{H}{\bf R}_{l}^{H})\big] \nonumber \\
&& + \mathbb{E}\big[{\rm tr}(\sum_{t=1}^{K_T}{\bf R}_{l}\boldsymbol{\Delta}_{tl}{\bf W}_{t}\boldsymbol{\Delta}_{tl}^{H}{\bf R}_{l}^{H})\big] \nonumber \\
\end{IEEEeqnarray}
The last two terms form a special case and can be solved using trace properties as given in lemma 1 in~\cite{}. Proof of the same is described in Sec.~\ref{app:mse:lemma}. Hence, the MSE for legitimate users is given as:
\begin{IEEEeqnarray}{lll}
&=& {\rm tr}({\bf I}) -%
{\rm tr}(\sum_{t=1}^{K_T}{\bf R}_{l}\widehat{\bf C}_{tl}{\bf V}_{t}) -%
{\rm tr}(\sum_{t=1}^{K_T}{\bf V}_{t}^{H}\widehat{\bf C}_{tl}^{H}{\bf R}_{l}^{H}) +%
{\rm tr}(\sum_{t=1}^{K_T}{\bf R}_{l}\widehat{\bf C}_{tl}{\bf V}_{t}{\bf V}_{t}^{H}\widehat{\bf C}_{tl}^{H}{\bf R}_{l}^{H}) + \nonumber \\%
&&\quad {\rm tr}(\sum_{t=1}^{K_T}{\bf R}_{l}\widehat{\bf C}_{tl}{\bf W}_{t}\widehat{\bf C}_{tl}^{H}{\bf R}_{l}^{H}) +%
{\sigma}_{nl}^{2}{\rm tr}({\bf R}_{l}{\bf R}_{l}^{H}) +%
\sum_{t=1}^{K_T}{\sigma}_{tl}^{2}{\rm tr}({\bf R}_{l}{\bf R}_{l}^{H}){\rm tr}({\bf V}_{t}{\bf V}_{t}^{H}) \nonumber \\%
&& + \sum_{t=1}^{K_T}{\sigma}_{tl}^{2}{\rm tr}({\bf R}_{l}{\bf R}_{l}^{H}){\rm tr}({\bf W}_{t})
\end{IEEEeqnarray}
\subsection{MSE at eavesdroppers}

\begin{IEEEeqnarray}{lll}
\label{eq:mse_eve_complete}
{\epsilon}_{e} &=& \mathbb{E}\bigg[||{\bf d}-\overline{\bf d}_{e}||^{2}\bigg] \nonumber
\\
&=&\mathbb{E}\bigg[||{\bf d}-(\sum_{t=1}^{K_T}{\bf E}_{e}(\widehat{\bf G}_{te} + \boldsymbol{\Delta}_{te}){\bf V}_{t}{\bf d} + \sum_{t=1}^{K_T}{\bf E}_{e}(\widehat{\bf G}_{te} + \boldsymbol{\Delta}_{te}){\bf w}_{t} + {\bf E}_{e}{\bf n}_{e})||^{2}\bigg]\nonumber \\
&=&\mathbb{E}\bigg[{\rm tr}\Big(({\bf d}-(\sum_{t=1}^{K_T}{\bf E}_{e}(\widehat{\bf G}_{te} + \boldsymbol{\Delta}_{te}){\bf V}_{t}{\bf d} + \sum_{t=1}^{K_T}{\bf E}_{e}(\widehat{\bf G}_{te} + \boldsymbol{\Delta}_{te}){\bf w}_{t} + {\bf E}_{e}{\bf n}_{e}))\nonumber \\
&&\qquad({\bf d}-(\sum_{t=1}^{K_T}{\bf E}_{e}(\widehat{\bf G}_{te} + \boldsymbol{\Delta}_{te}){\bf V}_{t}{\bf d} + \sum_{t=1}^{K_T}{\bf E}_{e}(\widehat{\bf G}_{te} + \boldsymbol{\Delta}_{te}){\bf w}_{t} + {\bf E}_{e}{\bf n}_{e}))^{H}\Big)\bigg]\nonumber \\
&=& \mathbb{E}\bigg[{\rm tr}\Big(%
{\bf d}{\bf d}^{H}-%
\sum_{t=1}^{K_T}{\bf E}_{e}(\widehat{\bf G}_{te} + \boldsymbol{\Delta}_{te}){\bf V}_{t}{\bf d}{\bf d}^{H} -%
\sum_{t=1}^{K_T}{\bf E}_{e}(\widehat{\bf G}_{te} + \boldsymbol{\Delta}_{te}){\bf w}_{t}{\bf d}^{H} -%
{\bf E}_{e}{\bf n}_{e}{\bf d}^{H} - \nonumber \\%
&&\quad \sum_{t=1}^{K_T}{\bf d}{\bf d}^{H}{\bf V}_{t}^{H}(\widehat{\bf G}_{te} + \boldsymbol{\Delta}_{te})^{H}{\bf E}_{e}^{H} +%
\sum_{t=1}^{K_T}{\bf E}_{e}(\widehat{\bf G}_{te} + \boldsymbol{\Delta}_{te}){\bf V}_{t}{\bf d}{\bf d}^{H}{\bf V}_{t}^{H}(\widehat{\bf G}_{te} + \boldsymbol{\Delta}_{te})^{H}{\bf E}_{e}^{H} \nonumber \\%
&&+ \sum_{t=1}^{K_T}{\bf E}_{e}(\widehat{\bf G}_{te} + \boldsymbol{\Delta}_{te}){\bf w}_{t}{\bf d}^{H}{\bf V}_{t}^{H}(\widehat{\bf G}_{te} + \boldsymbol{\Delta}_{te})^{H}{\bf E}_{e}^{H} +%
\sum_{t=1}^{K_T}{\bf E}_{e}{\bf n}_{e}{\bf d}^{H}{\bf V}_{t}^{H}(\widehat{\bf G}_{te} + \boldsymbol{\Delta}_{te})^{H}{\bf E}_{e}^{H} \nonumber \\%
&&- \sum_{t=1}^{K_T}{\bf d}{\bf w}_{t}^{H}(\widehat{\bf G}_{te} + \boldsymbol{\Delta}_{te})^{H}{\bf E}_{e}^{H} +%
\sum_{t=1}^{K_T}{\bf E}_{e}(\widehat{\bf G}_{te} + \boldsymbol{\Delta}_{te}){\bf V}_{t}{\bf d}{\bf w}_{t}^{H}(\widehat{\bf G}_{te} + \boldsymbol{\Delta}_{te})^{H}{\bf E}_{e}^{H} + \nonumber \\%
&&\quad \sum_{t=1}^{K_T}{\bf E}_{e}(\widehat{\bf G}_{te} + \boldsymbol{\Delta}_{te}){\bf w}_{t}{\bf w}_{t}^{H}(\widehat{\bf G}_{te} + \boldsymbol{\Delta}_{te})^{H}{\bf E}_{e}^{H} +%
\sum_{t=1}^{K_T}{\bf E}_{e}{\bf n}_{e}{\bf w}_{t}^{H}(\widehat{\bf G}_{te} + \boldsymbol{\Delta}_{te})^{H}{\bf E}_{e}^{H} -%
{\bf d}{\bf n}_{e}^{H}{\bf E}_{e}^{H} \nonumber \\
&&+ \sum_{t=1}^{K_T}{\bf E}_{e}(\widehat{\bf G}_{te} + \boldsymbol{\Delta}_{te}){\bf V}_{t}{\bf d}{\bf n}_{e}^{H}{\bf E}_{e}^{H} +%
\sum_{t=1}^{K_T}{\bf E}_{e}(\widehat{\bf G}_{te} + \boldsymbol{\Delta}_{te}){\bf w}_{t}{\bf n}_{e}^{H}{\bf E}_{e}^{H} +%
{\bf E}_{e}{\bf n}_{e}{\bf n}_{e}^{H}{\bf E}_{e}^{H}%
\Big)\bigg]\nonumber \\
&=& {\rm tr}({\bf I}) -%
{\rm tr}(\sum_{t=1}^{K_T}{\bf E}_{e}\widehat{\bf G}_{te}{\bf V}_{t}) -%
{\rm tr}(\sum_{t=1}^{K_T}{\bf V}_{t}^{H}\widehat{\bf G}_{te}^{H}{\bf E}_{e}^{H}) +%
{\rm tr}(\sum_{t=1}^{K_T}{\bf E}_{e}\widehat{\bf G}_{te}{\bf V}_{t}{\bf V}_{t}^{H}\widehat{\bf G}_{te}^{H}{\bf E}_{e}^{H}) + \nonumber \\%
&&\quad {\rm tr}(\sum_{t=1}^{K_T}{\bf E}_{e}\widehat{\bf G}_{te}{\bf W}_{t}\widehat{\bf G}_{te}^{H}{\bf E}_{e}^{H}) +%
{\sigma}_{ne}^{2}{\rm tr}({\bf E}_{e}{\bf E}_{e}^{H}) +%
\mathbb{E}\big[{\rm tr}(\sum_{t=1}^{K_T}{\bf E}_{e}\boldsymbol{\Delta}_{te}{\bf V}_{t}{\bf V}_{t}^{H}\boldsymbol{\Delta}_{te}^{H}{\bf E}_{e}^{H})\big] \nonumber \\
&& + \mathbb{E}\big[{\rm tr}(\sum_{t=1}^{K_T}{\bf E}_{e}\boldsymbol{\Delta}_{te}{\bf W}_{t}\boldsymbol{\Delta}_{te}^{H}{\bf E}_{e}^{H})\big] \nonumber \\
&=& {\rm tr}({\bf I}) -%
{\rm tr}(\sum_{t=1}^{K_T}{\bf E}_{e}\widehat{\bf G}_{te}{\bf V}_{t}) -%
{\rm tr}(\sum_{t=1}^{K_T}{\bf V}_{t}^{H}\widehat{\bf G}_{te}^{H}{\bf E}_{e}^{H}) +%
{\rm tr}(\sum_{t=1}^{K_T}{\bf E}_{e}\widehat{\bf G}_{te}{\bf V}_{t}{\bf V}_{t}^{H}\widehat{\bf G}_{te}^{H}{\bf E}_{e}^{H}) + \nonumber \\%
&&\quad {\rm tr}(\sum_{t=1}^{K_T}{\bf E}_{e}\widehat{\bf G}_{te}{\bf W}_{t}\widehat{\bf G}_{te}^{H}{\bf E}_{e}^{H}) +%
{\sigma}_{ne}^{2}{\rm tr}({\bf E}_{e}{\bf E}_{e}^{H}) +%
\sum_{t=1}^{K_T}{\sigma}_{te}^{2}{\rm tr}({\bf E}_{e}{\bf E}_{e}^{H}){\rm tr}({\bf V}_{t}{\bf V}_{t}^{H}) \nonumber \\%
&& + \sum_{t=1}^{K_T}{\sigma}_{te}^{2}{\rm tr}({\bf E}_{e}{\bf E}_{e}^{H}){\rm tr}({\bf W}_{t})
\end{IEEEeqnarray}
