# Supplementary material for: Secure and Robust MIMO Transceiver for Multicast Mission Critical Communications
Source: arXiv:2012.05829 source file (2020-12-10)
Supplement: Supplementary file 4 [file appendix_proposition1.tex]

A generalized solution for the design of secure transceivers is presented in this section. Two binary slack variables ${\chi}_{l}$ and ${\chi}_{e}$ are added to the optimization problem in order to maintain generality among different propositions. ${\chi}_{l} = 1$ corresponds to a robust solution for legitimate users and ${\chi}_{l} = 0$ otherwise. ${\chi}_{e} = 1$ is considered when the CSI of eavesdroppers in not perfectly known at transmitters, while ${\chi}_{e} = 0$ correlates to when transmitters have perfect knowledge of CSI of eavesdroppers. The generalized MSE equations are reformulated as:
\begin{IEEEeqnarray}{lll}
{\epsilon}_{l} &=& {\rm tr}({\bf I}) -%
{\rm tr}(\sum_{t=1}^{K_T}{\bf R}_{l}\widehat{\bf C}_{tl}{\bf V}_{t}) -%
{\rm tr}(\sum_{t=1}^{K_T}{\bf V}_{t}^{H}\widehat{\bf C}_{tl}^{H}{\bf R}_{l}^{H}) +%
{\rm tr}(\sum_{t=1}^{K_T}{\bf R}_{l}\widehat{\bf C}_{tl}{\bf V}_{t}{\bf V}_{t}^{H}\widehat{\bf C}_{tl}^{H}{\bf R}_{l}^{H}) \nonumber \\%
&&+ {\rm tr}(\sum_{t=1}^{K_T}{\bf R}_{l}\widehat{\bf C}_{tl}{\bf W}_{t}\widehat{\bf C}_{tl}^{H}{\bf R}_{l}^{H}) +%
{\sigma}_{nl}^{2}{\rm tr}({\bf R}_{l}{\bf R}_{l}^{H}) +%
{\chi}_{l}\sum_{t=1}^{K_T}{\sigma}_{tl}^{2}{\rm tr}({\bf R}_{l}{\bf R}_{l}^{H}){\rm tr}({\bf V}_{t}{\bf V}_{t}^{H}) \nonumber \\%
&&+ {\chi}_{l}\sum_{t=1}^{K_T}{\sigma}_{tl}^{2}{\rm tr}({\bf R}_{l}{\bf R}_{l}^{H}){\rm tr}({\bf W}_{t}) \label{eq:mse_leg_gen} \\
{\epsilon}_{e} &=& {\rm tr}({\bf I}) -%
{\rm tr}(\sum_{t=1}^{K_T}{\bf E}_{e}\widehat{\bf G}_{te}{\bf V}_{t}) -%
{\rm tr}(\sum_{t=1}^{K_T}{\bf V}_{t}^{H}\widehat{\bf G}_{te}^{H}{\bf E}_{e}^{H}) +%
{\rm tr}(\sum_{t=1}^{K_T}{\bf E}_{e}\widehat{\bf G}_{te}{\bf V}_{t}{\bf V}_{t}^{H}\widehat{\bf G}_{te}^{H}{\bf E}_{e}^{H}) \nonumber \\%
&& + {\rm tr}(\sum_{t=1}^{K_T}{\bf E}_{e}\widehat{\bf G}_{te}{\bf W}_{t}\widehat{\bf G}_{te}^{H}{\bf E}_{e}^{H}) +%
{\sigma}_{ne}^{2}{\rm tr}({\bf E}_{e}{\bf E}_{e}^{H}) +%
{\chi}_{e}\sum_{t=1}^{K_T}{\sigma}_{te}^{2}{\rm tr}({\bf E}_{e}{\bf E}_{e}^{H}){\rm tr}({\bf V}_{t}{\bf V}_{t}^{H}) \nonumber \\%
&& + {\chi}_{e}\sum_{t=1}^{K_T}{\sigma}_{te}^{2}{\rm tr}({\bf E}_{e}{\bf E}_{e}^{H}){\rm tr}({\bf W}_{t}) \label{eq:mse_eve_gen}
\end{IEEEeqnarray}
We solve the optimization problem~\eqref{eq:gen_opt} by formulating a Lagrange solution ${\rm L}$ which is given as:
\begin{IEEEeqnarray}{lll}
\label{eq:lagrange}
{\rm L}({\bf V}_{t}, {\bf W}_{t}, {\bf R}_{l}, {\lambda}_{e}, {\lambda}_{l}^{'}, {\lambda}_{l}^{''}) &=& \sum_{l=1}^{K_R}{\epsilon}_{l} - \sum_{e=1}^{K_E}{\lambda}_{e}({\epsilon}_{e} - \Gamma) + \sum_{t=1}^{K_T}{\lambda}_{t}^{'}({\rm tr}({\bf V}_{t}{\bf V}_{t}^{H} + {\bf W}_{t}) - P_T) \nonumber \\
&&- \sum_{t=1}^{K_T}{\lambda}_{t}^{''}({\rm tr}({\bf V}_{t}{\bf V}_{t}^{H}) - {\rm tr}({\bf W}_{t}))
\end{IEEEeqnarray}
The desired transceivers are obtained by minimizing the Lagrangian with respect to each optimization variable while considering that the other variables as fixed/known. Hence, the precoder $\{{\bf V}_{t}\}$ is derived by taking the zero gradient of ${\rm L}$ with respect to $\{{\bf V}_{t}^{H}\}$, and is given as. 
\begin{IEEEeqnarray}{lll}
\frac{\partial{\rm L}}{\partial{\bf V}_{t}^{H}} &=& - \sum_{l=1}^{K_R}\widehat{{\bf C}}_{tl}^{H}{\bf R}_{l}^{H} +%
\sum_{l=1}^{K_R}\widehat{{\bf C}}_{tl}^{H}{\bf R}_{l}^{H}{\bf R}_{l}\widehat{\bf C}_{tl}{\bf V}_{t} +%
{\chi}_{l}\sum_{l=1}^{K_R}{\sigma}_{tl}^{2}{\rm tr}({\bf R}_{l}{\bf R}_{l}^{H}){\bf V}_{t} +%
\sum_{e=1}^{K_E}{\lambda}_{e}\widehat{\bf G}_{te}^{H}{\bf E}_{e}^{H} - \nonumber \\%
&&\quad \sum_{e=1}^{K_E}{\lambda}_{e}\widehat{\bf G}_{te}^{H}{\bf E}_{e}^{H}{\bf E}_{e}\widehat{\bf G}_{te}{\bf V}_{t} -%
{\chi}_{e}\sum_{e=1}^{K_E}{\lambda}_{e}{\sigma}_{te}^{2}{\rm tr}({\bf E}_{e}{\bf E}_{e}^{H}){\bf V}_{t} +%
\lambda_{t}^{'}{\bf V}_{t} -%
\lambda_{t}^{''}{\bf V}_{t} = 0 \nonumber \\
\implies {\bf V}_{t} &=& \Big(\sum_{l=1}^{K_R}\widehat{{\bf C}}_{tl}^{H}{\bf R}_{l}^{H}{\bf R}_{l}\widehat{\bf C}_{tl} +%
{\chi}_{l}\sum_{l=1}^{K_R}{\sigma}_{tl}^{2}{\rm tr}({\bf R}_{l}{\bf R}_{l}^{H}){\bf I} - 
\sum_{e=1}^{K_E}{\lambda}_{e}\widehat{\bf G}_{te}^{H}{\bf E}_{e}^{H}{\bf E}_{e}\widehat{\bf G}_{te} - \nonumber \\%
&&\quad {\chi}_{e}\sum_{e=1}^{K_E}{\lambda}_{e}{\sigma}_{te}^{2}{\rm tr}({\bf E}_{e}{\bf E}_{e}^{H}){\bf I} +%
\lambda_{t}^{'}{\bf I} -%
\lambda_{t}^{''}{\bf I}
\Big)^{-1}{\Big(\sum_{l=1}^{K_R}\widehat{{\bf C}}_{tl}^{H}{\bf R}_{l}^{H} -%
\sum_{e=1}^{K_E}{\lambda}_{e}\widehat{\bf G}_{te}^{H}{\bf E}_{e}^{H} \Big)} \label{eq:precoder_gen}
\end{IEEEeqnarray}
Receive filter $\{{\bf R}_{l}\}$ is obtained in the same way, i.e. by differentiating Lagrangian with respect to ${\bf R}_{l}^{H}$, while considering all other variables as fixed, and assigning it to zero we get:
\begin{IEEEeqnarray}{lll}
\frac{\partial{\rm L}}{\partial{\bf R}_{l}^{H}} &=& - \sum_{t=1}^{K_T}{\bf V}_{t}^{H}\widehat{{\bf C}}_{tl}^{H} +%
\sum_{t=1}^{K_T}{\bf R}_{l}\widehat{{\bf C}}_{tl}{\bf V}_{t}{\bf V}_{t}^{H}\widehat{{\bf C}}_{tl}^{H} +%
\sum_{t=1}^{K_T}{\bf R}_{l}\widehat{{\bf C}}_{tl}{\bf W}_{t}\widehat{{\bf C}}_{tl}^{H} +%
{\sigma}_{nl}^{2}{\bf R}_{l} + \nonumber \\%
&&\quad {\chi}_{l}\sum_{t=1}^{K_T}{\sigma}_{tl}^{2}{\rm tr}({\bf V}_{t}{\bf V}_{t}^{H}){\bf R}_{l} +%
{\chi}_{l}\sum_{t=1}^{K_T}{\sigma}_{tl}^{2}{\rm tr}({\bf W}_{t}){\bf R}_{l} \nonumber \\
\implies {\bf R}_{l} &=& \Big(\sum_{t=1}^{K_T}{\bf V}_{t}^{H}\widehat{{\bf C}}_{tl}^{H}\Big)\Big(\sum_{t=1}^{K_T}\widehat{{\bf C}}_{tl}{\bf V}_{t}{\bf V}_{t}^{H}\widehat{{\bf C}}_{tl}^{H} +%
\sum_{t=1}^{K_T}\widehat{{\bf C}}_{tl}{\bf W}_{t}\widehat{{\bf C}}_{tl}^{H} + {\sigma}_{nl}^{2}{\bf I} +\nonumber \\%
&&\quad {\chi}_{l}\sum_{t=1}^{K_T}{\sigma}_{tl}^{2}{\rm tr}({\bf V}_{t}{\bf V}_{t}^{H}){\bf I} +%
{\chi}_{l}\sum_{t=1}^{K_T}{\sigma}_{tl}^{2}{\rm tr}({\bf W}_{t}){\bf I} \Big)^{-1} \label{eq:receiver_gen}
\end{IEEEeqnarray}
Now, we differentiate Lagrangian with ${\bf W}_{t}$ and assigning it to zero,
\begin{IEEEeqnarray}{lll}
\label{eq:lambda_1}
\frac{\partial{\rm L}}{\partial{\bf W}_{t}} &=& \sum_{l=1}^{K_R}\widehat{{\bf C}}_{tl}^{H}{\bf R}_{l}^{H}{\bf R}_{l}\widehat{\bf C}_{tl} +%
{\chi}_{l}\sum_{l=1}^{K_R}{\sigma}_{tl}^{2}{\rm tr}({\bf R}_{l}{\bf R}_{l}^{H}){\bf I} -% 
\sum_{e=1}^{K_E}{\lambda}_{e}\widehat{\bf G}_{te}^{H}{\bf E}_{e}^{H}{\bf E}_{e}\widehat{\bf G}_{te} -\nonumber \\%
&&\quad {\chi}_{e}\sum_{e=1}^{K_E}{\lambda}_{e}{\sigma}_{te}^{2}{\rm tr}({\bf E}_{e}{\bf E}_{e}^{H}){\bf I} +%
\lambda_{t}^{'}{\bf I} +%
\lambda_{t}^{''}{\bf I} = 0
\end{IEEEeqnarray}
Further, differentiating Lagrangian with  $\lambda_{e}$, $\lambda_{t}^{'}$, and $\lambda_{t}^{''}$ respectively. After equating it to zero, we get:
\begin{IEEEeqnarray}{lll}
\frac{\partial{\rm L}}{\partial{\lambda_{t}^{'}}} &=& {\rm tr}({\bf V}_{t}{\bf V}_{t}^{H} + {\bf W}_{t}) - P_{T} = 0 \label{eq:lambda_2}\\
\frac{\partial{\rm L}}{\partial{\lambda_{t}^{''}}} &=& {\rm tr}({\bf V}_{t}{\bf V}_{t}^{H}) - {\rm tr}({\bf W}_{t}) = 0 \label{eq:lambda_3}\\
\frac{\partial{\rm L}}{\partial{\lambda_{e}}} &=&
{\epsilon}_e - \Gamma = 0 \label{eq:W_noise}
\end{IEEEeqnarray}
The values for $\lambda_{e}$, $\lambda_{t}^{'}$, and $\lambda_{t}^{''}$ is computed by solving the set of linear equations using~\eqref{eq:lambda_1},~\eqref{eq:lambda_2}, and~\eqref{eq:lambda_3}. We consider these equations by taking the equation of ${\bf V}_{t}$ as in~\eqref{eq:precoder_gen} and sum over all the values of $t=1,2,\cdots,K_T$. Final set of equations can be written as:
\begin{IEEEeqnarray}{lll}
\label{eq:lambda_eqns}
&&\sum_{t=1}^{K_T}\sum_{l=1}^{K_R}\widehat{{\bf C}}_{tl}^{H}{\bf R}_{l}^{H}{\bf R}_{l}\widehat{\bf C}_{tl} +%
{\chi}_{l}\sum_{t=1}^{K_T}\sum_{l=1}^{K_R}{\sigma}_{tl}^{2}{\rm tr}({\bf R}_{l}{\bf R}_{l}^{H}){\bf I} -% 
\sum_{t=1}^{K_T}\sum_{e=1}^{K_E}{\lambda}_{e}\widehat{\bf G}_{te}^{H}{\bf E}_{e}^{H}{\bf E}_{e}\widehat{\bf G}_{te} +%
\sum_{t=1}^{K_T}\lambda_{t}^{'}{\bf I} - \nonumber \\  
&&{\chi}_{e}\sum_{t=1}^{K_T}\sum_{e=1}^{K_E}{\lambda}_{e}{\sigma}_{te}^{2}{\rm tr}({\bf E}_{e}{\bf E}_{e}^{H}){\bf I} +%
\sum_{t=1}^{K_T}\lambda_{t}^{''}{\bf I} = 0 \nonumber \\
&&\sum_{t=1}^{K_T}{\rm tr}({\bf V}_{t}{\bf V}_{t}^{H}) + \sum_{t=1}^{K_T}{\rm tr}({\bf W}_{t}) = \sum_{t=1}^{K_T}P_{T} \nonumber \\
&&\sum_{t=1}^{K_T}{\rm tr}({\bf V}_{t}{\bf V}_{t}^{H}) = \sum_{t=1}^{K_T}{\rm tr}({\bf W}_{t})\nonumber
\end{IEEEeqnarray}
Added noise factor ${\bf W}_{t}$ is derived using~\eqref{eq:W_noise} by taking the sum over all the values of $e=1,2,\cdots,K_E$ and reformulating it as:
\begin{IEEEeqnarray}{lll}
\label{eq:W_noise_eqns}
&&\sum_{e=1}^{K_E}{\epsilon}_{e} = \sum_{e=1}^{K_E}{\Gamma}\nonumber \\
&&\sum_{e=1}^{K_E}{\rm tr}({\bf I}) -%
\sum_{e=1}^{K_E}\sum_{t=1}^{K_T}{\rm tr}({\bf E}_{e}\widehat{\bf G}_{te}{\bf V}_{t}) -%
\sum_{e=1}^{K_E}\sum_{t=1}^{K_T}{\rm tr}({\bf V}_{t}^{H}\widehat{\bf G}_{te}^{H}{\bf E}_{e}^{H}) +%
\sum_{e=1}^{K_E}\sum_{t=1}^{K_T}{\rm tr}({\bf E}_{e}\widehat{\bf G}_{te}{\bf V}_{t}{\bf V}_{t}^{H}\widehat{\bf G}_{te}^{H}{\bf E}_{e}^{H}) \nonumber \\%
&& + \sum_{e=1}^{K_E}\sum_{t=1}^{K_T}{\rm tr}({\bf E}_{e}\widehat{\bf G}_{te}{\bf W}_{t}\widehat{\bf G}_{te}^{H}{\bf E}_{e}^{H}) +%
\sum_{e=1}^{K_E}{\sigma}_{ne}^{2}{\rm tr}({\bf E}_{e}{\bf E}_{e}^{H}) +%
{\chi}_{e}\sum_{e=1}^{K_E}\sum_{t=1}^{K_T}{\sigma}_{te}^{2}{\rm tr}({\bf E}_{e}{\bf E}_{e}^{H}){\rm tr}({\bf V}_{t}{\bf V}_{t}^{H}) \nonumber \\%
&& + {\chi}_{e}\sum_{e=1}^{K_E}\sum_{t=1}^{K_T}{\sigma}_{te}^{2}{\rm tr}({\bf E}_{e}{\bf E}_{e}^{H}){\rm tr}({\bf W}_{t}) \Big) = \sum_{e=1}^{K_E}{\Gamma} \nonumber \\
&& \sum_{e=1}^{K_E}\sum_{t=1}^{K_T}{\rm tr}({\bf E}_{e}\widehat{\bf G}_{te}{\bf W}_{t}\widehat{\bf G}_{te}^{H}{\bf E}_{e}^{H}) + {\chi}_{e}\sum_{e=1}^{K_E}\sum_{t=1}^{K_T}{\sigma}_{te}^{2}{\rm tr}({\bf E}_{e}{\bf E}_{e}^{H}){\rm tr}({\bf W}_{t}) = \nonumber \\%
&&\qquad \sum_{e=1}^{K_E}{\Gamma} -%
\sum_{e=1}^{K_E}{\rm tr}({\bf I}) +%
\sum_{e=1}^{K_E}\sum_{t=1}^{K_T}{\rm tr}({\bf E}_{e}\widehat{\bf G}_{te}{\bf V}_{t}) +%
\sum_{e=1}^{K_E}\sum_{t=1}^{K_T}{\rm tr}({\bf V}_{t}^{H}\widehat{\bf G}_{te}^{H}{\bf E}_{e}^{H}) -%
\sum_{e=1}^{K_E}{\sigma}_{ne}^{2}{\rm tr}({\bf E}_{e}{\bf E}_{e}^{H}) - \nonumber \\%
&&\qquad\sum_{e=1}^{K_E}\sum_{t=1}^{K_T}{\rm tr}({\bf E}_{e}\widehat{\bf G}_{te}{\bf V}_{t}{\bf V}_{t}^{H}\widehat{\bf G}_{te}^{H}{\bf E}_{e}^{H}) -%
{\chi}_{e}\sum_{e=1}^{K_E}\sum_{t=1}^{K_T}{\sigma}_{te}^{2}{\rm tr}({\bf E}_{e}{\bf E}_{e}^{H}){\rm tr}({\bf V}_{t}{\bf V}_{t}^{H}) \nonumber
\end{IEEEeqnarray}
Solving it for $t^{th}$ BS, Let the term in right hand side be $A_{t}$ such that,
\begin{IEEEeqnarray}{lll}
&&{A}_{t} = \sum_{e=1}^{K_E}{\Gamma} -%
\sum_{e=1}^{K_E}{\rm tr}({\bf I}) +%
\sum_{e=1}^{K_E}{\rm tr}({\bf E}_{e}\widehat{\bf G}_{te}{\bf V}_{t}) +%
\sum_{e=1}^{K_E}{\rm tr}({\bf V}_{t}^{H}\widehat{\bf G}_{te}^{H}{\bf E}_{e}^{H}) -%
\sum_{e=1}^{K_E}{\sigma}_{ne}^{2}{\rm tr}({\bf E}_{e}{\bf E}_{e}^{H}) - \nonumber \\%
&&\qquad\sum_{e=1}^{K_E}{\rm tr}({\bf E}_{e}\widehat{\bf G}_{te}{\bf V}_{t}{\bf V}_{t}^{H}\widehat{\bf G}_{te}^{H}{\bf E}_{e}^{H}) -%
{\chi}_{e}\sum_{e=1}^{K_E}{\sigma}_{te}^{2}{\rm tr}({\bf E}_{e}{\bf E}_{e}^{H}){\rm tr}({\bf V}_{t}{\bf V}_{t}^{H}) \nonumber
\end{IEEEeqnarray}
Hence,
\begin{IEEEeqnarray}{lll}
&&\sum_{e=1}^{K_E}{\rm tr}({\bf E}_{e}\widehat{\bf G}_{te}{\bf W}_{t}\widehat{\bf G}_{te}^{H}{\bf E}_{e}^{H}) + {\chi}_{e}\sum_{e=1}^{K_E}{\sigma}_{te}^{2}{\rm tr}({\bf E}_{e}{\bf E}_{e}^{H}){\rm tr}({\bf W}_{t}) = {A}_{t} \nonumber \\
&&\sum_{e=1}^{K_E}{\rm tr}(\widehat{\bf G}_{te}^{H}{\bf E}_{e}^{H}{\bf E}_{e}\widehat{\bf G}_{te}{\bf W}_{t}) + {\chi}_{e}\sum_{e=1}^{K_E}{\sigma}_{te}^{2}{\rm tr}({\bf E}_{e}{\bf E}_{e}^{H}){\rm tr}({\bf I}{\bf W}_{t}) = {A}_{t} \nonumber
\end{IEEEeqnarray}
Using the trace property ${\rm tr}(AB) = {\rm vec}(A^{T})^{T}{\rm vec}(B)$, above equation can be written as:
\begin{IEEEeqnarray}{lll}
&&\sum_{e=1}^{K_E}\big({\rm vec}(\widehat{\bf G}_{te}^{H}{\bf E}_{e}^{H}{\bf E}_{e}\widehat{\bf G}_{te})^{H}{\rm vec}({\bf W}_{t})\big) + {\chi}_{e}\sum_{e=1}^{K_E}{\sigma}_{te}^{2}{\rm tr}({\bf E}_{e}{\bf E}_{e}^{H}){\rm vec}({\bf I})^{H}{\rm vec}({\bf W}_{t}) = {A}_{t} \nonumber \\
&&\Big(\sum_{e=1}^{K_E}{\rm vec}(\widehat{\bf G}_{te}^{H}{\bf E}_{e}^{H}{\bf E}_{e}\widehat{\bf G}_{te})^{H} + {\chi}_{e}\sum_{e=1}^{K_E}{\sigma}_{te}^{2}{\rm tr}({\bf E}_{e}{\bf E}_{e}^{H}){\rm vec}({\bf I})^{H}\Big)\sum_{e=1}^{K_E}{\rm vec}({\bf W}_{t}) = {A}_{t} \nonumber \\
&&\Big(\sum_{e=1}^{K_E}{\rm vec}(\widehat{\bf G}_{te}^{H}{\bf E}_{e}^{H}{\bf E}_{e}\widehat{\bf G}_{te}) + {\chi}_{e}\sum_{e=1}^{K_E}{\sigma}_{te}^{2}{\rm tr}({\bf E}_{e}{\bf E}_{e}^{H}){\rm vec}({\bf I})\Big)^{H}\sum_{e=1}^{K_E}{\rm vec}({\bf W}_{t}) = {A}_{t} \nonumber \\
&&{\bf b}_{t}^{H}\sum_{e=1}^{K_E}{\rm vec}({\bf W}_{t}) = {A}_{t} \nonumber
\end{IEEEeqnarray}
where,
\begin{IEEEeqnarray}{lll}
{\bf b}_{t}^{H} = \sum_{e=1}^{K_E}{\rm vec}(\widehat{\bf G}_{te}^{H}{\bf E}_{e}^{H}{\bf E}_{e}\widehat{\bf G}_{te}) + {\chi}_{e}\sum_{e=1}^{K_E}{\sigma}_{te}^{2}{\rm tr}({\bf E}_{e}{\bf E}_{e}^{H}){\rm vec}({\bf I})
\end{IEEEeqnarray}
Pre-multiplying with ${\bf b}_{t}$ on both sides.
\begin{IEEEeqnarray}{lll}
&&{\bf b}_{t}{\bf b}_{t}^{H}\sum_{e=1}^{K_E}{\rm vec}({\bf W}_{t}) = {\bf b}_{t}{A}_{t} \nonumber \\
&&{\bf B}_{t}\sum_{e=1}^{K_E}{\rm vec}({\bf W}_{t}) = {\bf b}_{t}{A}_{t} \nonumber \\
&&{K_E}{\rm vec}({\bf W}_{t}) = {\bf B}_{t}^{-1}{\bf b}_{t}{A}_{t} \nonumber \\
&&{\rm vec}({\bf W}_{t}) = \frac{1}{{K_E}}{\bf B}_{t}^{-1}{\bf b}_{t}{A}_{t} \nonumber
\end{IEEEeqnarray}
Therefore, the matrix ${\bf W}_{t}$ is computed by performing matricization operation on the computed vector, i.e:
\begin{IEEEeqnarray}{lll}
\label{eq:W_final}
{\bf W}_{t} = {\rm mat}({\rm vec}({\bf W}_{t}))
\end{IEEEeqnarray}
